# Supplementary material for: Inferring rotations using a bosonic Josephson junction
Source: arXiv:2601.13344 ancillary file (2026-01-19)
Supplement: Supplementary file 1 [file Supplementary_material.pdf]

# Inferring rotations using a bosonic Josephson junction (Supplementary material)

Rhombik Roy[1,2,*] and Ofir E. Alon[1,2]

[1]*Department of Physics, University of Haifa, Haifa 3498838, Israel*

[2]*Haifa Research Center for Theoretical Physics and Astrophysics, University of Haifa, Haifa 3498838, Israel*

In this supplementary material, we present the convergence analysis of the numerical results with respect to two key parameters: the number of time-adaptive orbitals employed in the many-body calculations and the spatial grid resolution. Convergence is quantified using the occupations of the natural orbitals, as well as the variances of the transverse momentum and the angular momentum. While the main text examines the dynamics of the average transverse momentum and angular momentum in detail, primarily within a mean-field framework, here we also analyze the corresponding variances from a many-body perspective. This allows us to explicitly demonstrate the role of many-body correlations in these observables.

## I. CONVERGENCE OF THE OUT-OF-EQUILIBRIUM DYNAMICS AND ITS ANALYSIS

In this section, we analyze the convergence of the results presented in the main text. Convergence in many-body dynamics is crucial, as the time evolution involves contributions from multiple excited states [1–4].

In the main text, we discuss three main scenarios. First, the double well is placed at the center of the rotation axis. Second, the double well is shifted by a distance $S$ from the rotation center. Third, for an off-centered double well, we investigate how its orientation affects the tunneling dynamics. In all three cases, we analyze how tunneling is affected and how the rotation frequency or displacement can be inferred from the observables. Finally, we consider a scenario in which the double well rotates with time-dependent frequencies, allowing us to study additional rotation effects directly in the laboratory frame. All calculations in the main text are performed using $64 \times 64$ grid points, and the many-body simulations employ $N = 10$ bosons and $M = 8$ orbitals. Here, we examine the convergence of each scenario with respect to both the number of orbitals

* rroy@campus.haifa.ac.il

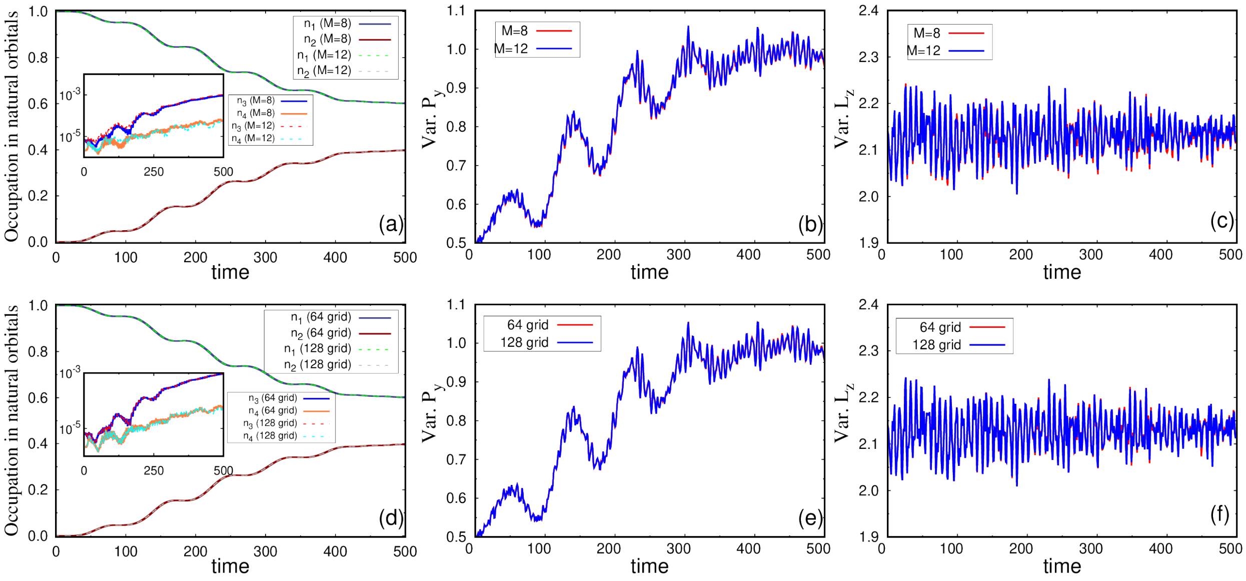


FIG. S1. (a–c) Convergence with respect to the number of orbitals and (d–f) convergence with respect to the grid resolution for the rotation axis passing through the center of the double well. Panels (a), (b), and (c) show, respectively, the time evolution of the occupations in the first four natural orbitals, the momentum variance $\frac{1}{N}\Delta^2_{P_y}(t)$, and the angular-momentum variance $\frac{1}{N}\Delta^2_{L_z}(t)$, computed with $M = 8$ and $M = 12$ orbitals for $\Omega = 0.15$. The very close overlap in all three cases confirms that $M = 8$ orbitals are sufficient for converged results. Panels (d), (e), and (f) present the same observables computed on $64 \times 64$ and $128 \times 128$ grid points, demonstrating that results for $64 \times 64$ grid points are sufficient to achieve convergence. All quantities are dimensionless.

and the number of grid points. In all cases, the interaction parameter is taken as $\Lambda = 0.2$. We find that the tunneling time, the self-trapping fraction, the amplitude of the transverse-momentum oscillations, and the time-averaged angular momentum are particularly sensitive to the tunneling dynamics under rotation.

Figure S1 presents the convergence analysis with respect to both the number of orbitals and the grid resolution for the case where the double well is centered at the origin ($S = 0$). For illustration, we use $\Omega = 0.15$. Figures S1(a) and (d) show the populations of the first two natural orbitals, with the third and fourth orbital occupations displayed in the insets. Figure S1(a) compares the time evolution of the first four natural orbital occupations obtained using $M = 8$ (solid) and $M = 12$ (dotted) orbitals. The curves lie on top of each other, indicating that increasing the number of orbitals from 8 to 12 does not alter the dynamics. This confirms that $M = 8$ orbitals are sufficient for converged results. We also observe that the occupations of the third and fourth orbitals are initially very small but increase as time progresses.

Similarly, Fig. S1(d) compares results obtained with $64 \times 64$ (solid) and $128 \times 128$ (dotted) grid points. The close overlap between the two resolutions demonstrates that a $64 \times 64$ grid points already yields converged results.

As an additional convergence check, we examine the variances of the transverse momentum and the angular momentum. These quantities are especially informative because they are highly sensitive to many-body correlations [5, 6]. The variance per particle of an operator $\hat{A}$, denoted by $\frac{1}{N}\Delta^2_{\hat{A}}$, is defined as

$$\frac{1}{N}\Delta^2_{\hat{A}} = \frac{1}{N}\langle\Psi(t)|\hat{A}^2|\Psi(t)\rangle - \frac{1}{N}\langle\Psi(t)|\hat{A}|\Psi(t)\rangle^2. \tag{1.1}$$

The first term, $\langle\hat{A}^2\rangle$, comprises both one-body and two-body contributions, expressed as $\hat{A}^2 = \sum_{j=1}^{N} \hat{a}_j^2 + \sum_{k>j=1}^{N} 2\hat{a}_j\hat{a}_k$, where $\hat{a}$ represents the corresponding single-particle operator. The second term of Eq. 1.1 involves only one-body contributions. For more details, see Refs. [5, 6].

Figures S1(b) and S1(e) show the variance of the momentum in the $y$-direction, $\frac{1}{N}\Delta^2_{\hat{P}_y}$, for different numbers of orbitals and grid sizes, respectively. The quantitative agreement between the $M = 8$ and $M = 12$ orbital simulations [Fig. S1(b)] as well as between the $64 \times 64$ and $128 \times 128$ grids [Fig. S1(e)] further confirms the convergence with $M = 8$ and $64 \times 64$ grid points. We also observe that as fragmentation increases, the transverse momentum distribution broadens, which is reflected in the growth of $\frac{1}{N}\Delta\hat{P}_y^2$.

Finally, Figures S1(c) and S1(f) show the variance of the angular momentum, $\frac{1}{N}\Delta^2_{\hat{L}_z}$, for the same convergence tests. The overlapping results between the $M = 8$ and $M = 12$ curves, as well as between the two grid resolutions, again confirms the convergence. The relatively large values and oscillatory behavior of $\frac{1}{N}\Delta\hat{L}_z^2$ capture the out-of-equilibrium rotational fluctuations that accompany the onset of fragmentation.

Next, we analyze the convergence of the results when the double well is displaced by an amount $S$ from the rotation axis ($S \neq 0, \theta = 0$; see Fig.3(a) of the main text). For illustration, we consider $S = 4$ and a slow rotation frequency $\Omega = 0.01$. Despite the small value of $\Omega$, such a rotation has a significant effect on the tunneling dynamics at this displacement. Similar to the previous case, Fig. S2 presents the convergence tests with respect to both the number of orbitals and the grid resolution. Figures S2(a) and S2(d) show the time evolution of the occupations in the first four natural orbitals computed with $M = 8$ and $M = 12$ orbitals and with $64 \times 64$ and $128 \times 128$ grid points, respectively. In both comparisons, the curves corresponding to the higher configurations lie on top of those from the lower configurations. This demonstrates that $M = 8$ orbitals and a $64 \times 64$ grid are sufficient to obtain converged results for the off-centered double well under rotation.

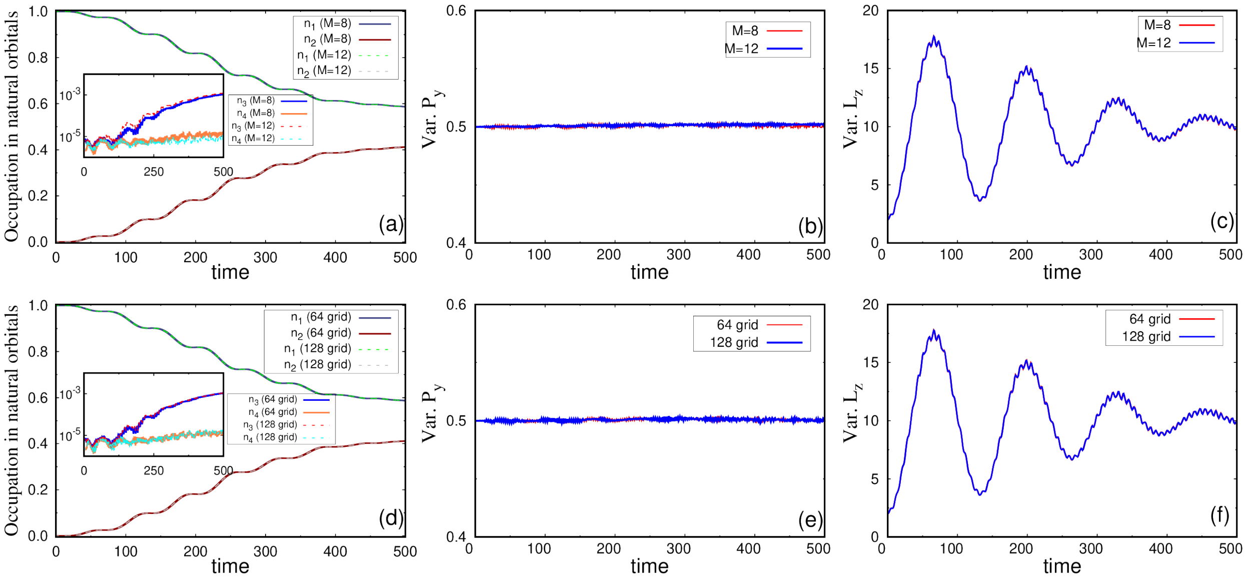


FIG. S2. (a–c) Convergence test with respect to the number of time-adaptive orbitals, and (d–f) convergence with respect to grid resolution, for the double well displaced from the rotation axis ($S = 4$, $\theta = 0$). Results are shown for $S = 4$ and $\Omega = 0.01$. Panels (a), (b), and (c) display the time evolution of the occupations in the first four natural orbitals, $\frac{1}{N}\Delta^2_{P_y}(t)$, and $\frac{1}{N}\Delta^2_{L_z}(t)$ computed with $M = 8$ and $M = 12$ orbitals. The system starts from a highly condensed state, and the depletion increases over time. The overlapping results between $M = 8$ and $M = 12$ confirms that results with $M = 8$ orbitals are converged. Panels (d), (e), and (f) show the same quantities computed using $64 \times 64$ and $128 \times 128$ grid points. The good agreement between the two resolutions demonstrates the convergence of the observables with $64 \times 64$ grid points. All quantities are dimensionless.

Figures S2(b), (c), (e), and (f) display these variances for both lower and higher numbers of orbitals, as well as for smaller and larger grid densities. The close agreement between the results obtained with higher and lower configurations further confirms the convergence of the results. The momentum variance $\frac{1}{N}\Delta^2_{P_y}(t)$ remains nearly flat, indicating that it is more sensitive to the rotation frequency than to the displacement $S$, and that no significant transverse excitations occur at this small $\Omega$. In contrast, the angular momentum variance $\frac{1}{N}\Delta^2_{L_z}(t)$ exhibits oscillations with relatively large amplitude, reflecting the non-equilibrium rotational fluctuations in the system.

Figure S3 shows the convergence analysis for the off-centered double well with the tunneling direction rotated by an angle $\theta$ with respect to the radial direction of rotation (see Fig.5(a) of the main text). For illustration, we consider $S = 4$, $\Omega = 0.015$, and $\theta = \pi/3$. Figures S3(a) and S3(d) compare results for $M = 8$ versus $M = 12$ time-adaptive orbitals and for grid resolution of $64 \times 64$ and $128 \times 128$. The very close agreement confirms that $M = 8$ orbitals and a $64 \times 64$

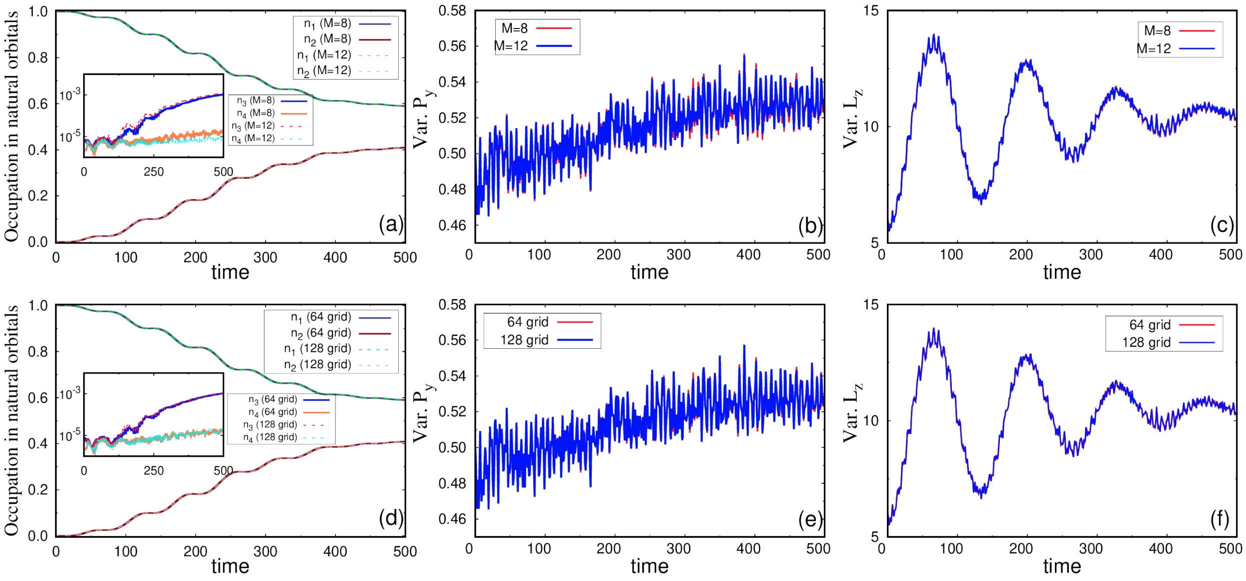


FIG. S3. (a–c) Convergence check with respect to the number of orbitals and (d–f) convergence check with respect to the grid resolution for a double well displaced from the rotation axis ($S = 4$) and rotated by an angle $\theta = \pi/3$. Panels (a), (b), and (c) show the time evolution of the first four natural orbital occupations, $\frac{1}{N}\Delta^2_{P_y}(t)$, and $\frac{1}{N}\Delta^2_{L_z}(t)$, respectively, computed with $M = 8$ and $M = 12$ orbitals. The initial state is highly condensed, and the depletion increases over time. In all observables, the $M = 8$ and $M = 12$ results overlap, demonstrating the convergence with $M = 8$ orbitals. Panels (d), (e), and (f) show the same quantities computed with $64 \times 64$ and $128 \times 128$ grid points, which again coincide, confirming convergence with respect to the $64 \times 64$ grid points. All quantities are dimensionless.

grid are sufficient to obtain converged results in this scenario. Similar convergence is observed in the variances of momentum along the y-direction ($\frac{1}{N}\Delta^2_{P_y}(t)$) and angular momentum ($\frac{1}{N}\Delta^2_{L_z}(t)$), where results for lower numerical resolutions lie on top of those from higher numerical resolutions [see Fig. S2(b), (c), (e), and (f)].

From a physical perspective, at this small rotation, $\frac{1}{N}\Delta^2_{P_y}(t)$ shows a slight increase over time, indicating the gradual development of transverse momentum fluctuations. In contrast, the angular momentum variance exhibits oscillatory behavior, reflecting persistent out-of-equilibrium rotational dynamics.

Lastly, we demonstrate the convergence of the time-dependent trap-rotation scenario, in which the trap is set into rotation with different switching times. We analyze the survival probability, as well as the time evolution of the transverse momentum and the angular momentum, for various switching times. The mean-field results in the main text are performed on a spatial domain from $-8$ to $+8$ in both the x and y directions, using $64 \times 64$ grid points. To assess the convergence with

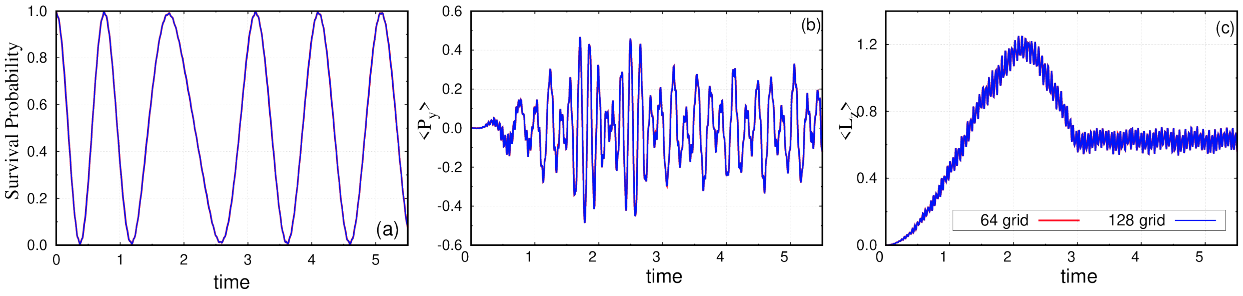


FIG. S4. Convergence of the trap-rotation dynamics with respect to the spatial grid density for a switching time of $\tau = 3T$ and rotation frequency $\Omega_{\text{final}} = 0.15$. Shown are the time evolutions of (a) the survival probability, (b) the expectation value of the transverse momentum per particle in the y direction, and (c) the angular momentum per particle. Results obtained using $64 \times 64$ grids (red) are compared with $128 \times 128$ grids (blue). The excellent agreement demonstrates that the numerical results are converged with respect to the grid resolution. All quantities shown are dimensionless.

respect to the grid density, we recalculate the same three quantities on a denser $128 \times 128$ grid and compare the results.

We find that, for all switching times considered, the $64 \times 64$ grid is sufficient to obtain converged results. As a representative example, we present results for a switching time of $\tau = 3T$ and final rotation frequency $\Omega_{\text{final}} = 0.15$, shown in Fig. S4. The survival probability [Fig. S4(a)], the expectation value of the transverse momentum per particle in the y direction [Fig. S4(b)], and the angular momentum per particle [Fig. S4(c)] exhibit excellent agreement in their time evolutions between calculations performed with $64 \times 64$ (blue curves) and $128 \times 128$ (red curves) grids. This agreement confirms that the numerical results presented in this work are well converged with respect to the spatial grid density.

## II. MANY-BODY EFFECTS IN THE MOMENTUM AND ANGULAR MOMENTUM OUT-OF-EQUILIBRIUM DYNAMICS

The main text primarily focuses on the mean-field dynamics of the transverse momentum and angular momentum. In this section, we examine the many-body effects on these quantities during the dynamics. As indicated by the convergence analysis of the natural orbital occupations, the system initially starts in a highly condensed state and gradually becomes fragmented over time. In the main text, we observe that when the mean-field survival probability exhibits full oscillations, the corresponding many-body survival probability shows oscillations with a decaying amplitude. This behavior is attributed to the onset of fragmentation. To illustrate the many-body behavior

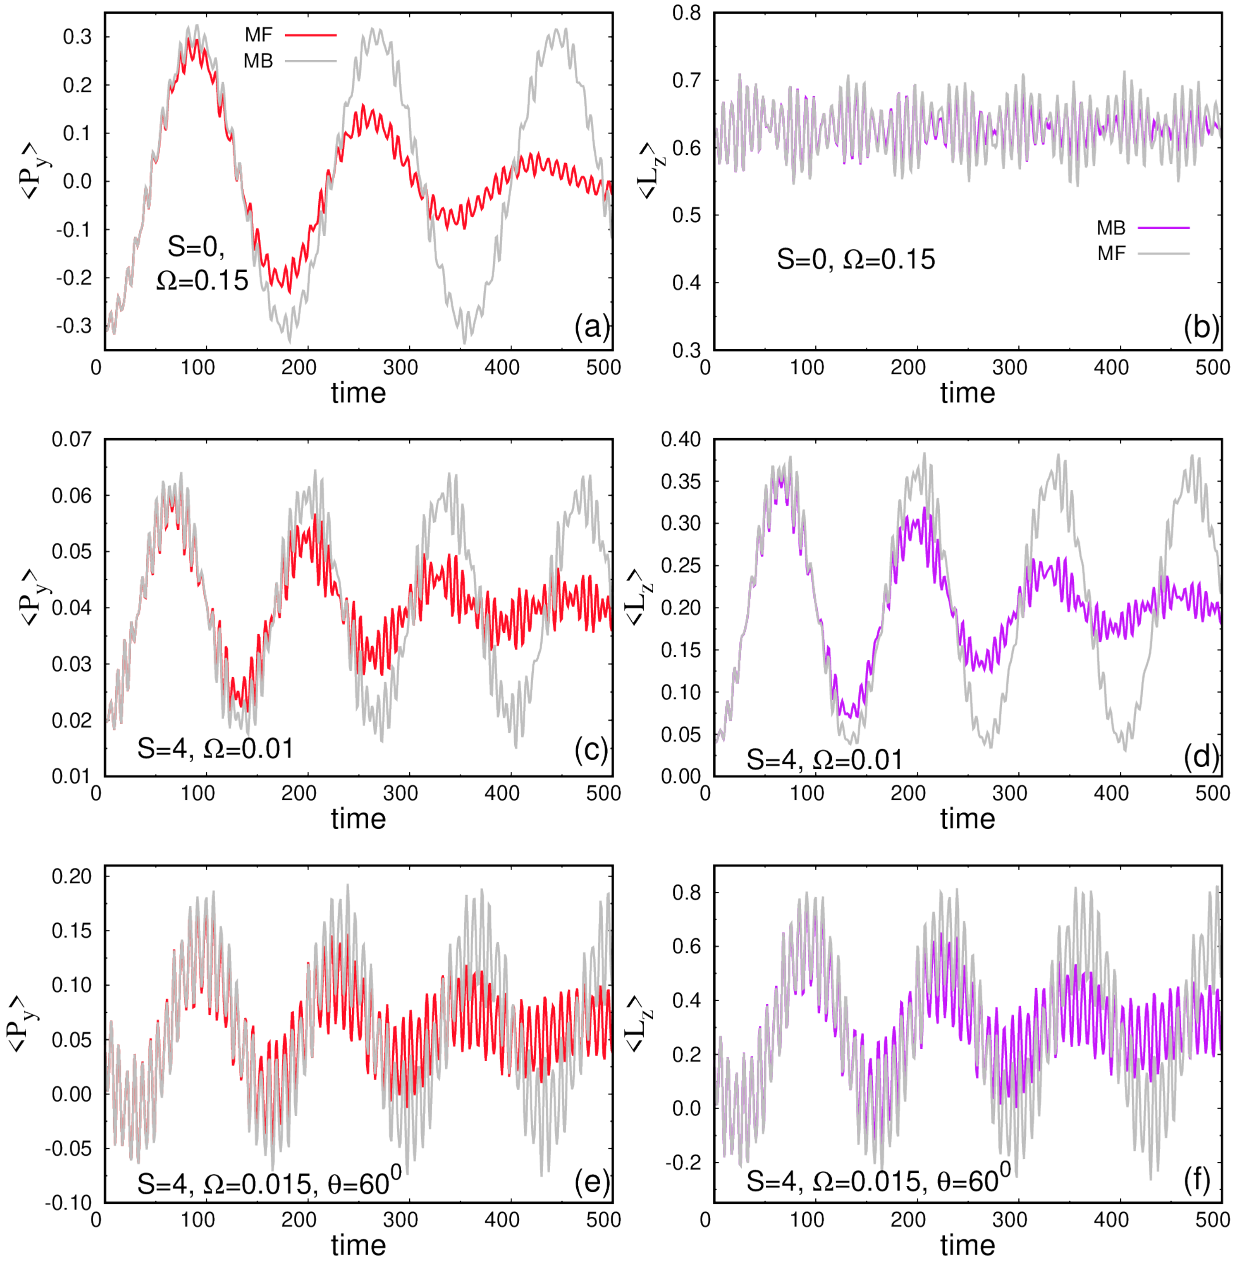


FIG. S5. Expectation values of the transverse momentum per particle (left column) and the average angular momentum per particle (right column) as functions of time. Results are shown for three configurations: (a,b) centered double-well potential and $\Omega = 0.15$; (c,d) double well displaced by $S = 4$ from the center and $\Omega = 0.01$; and (e,f) double well displaced by $S = 4$ and rotated by $\theta = 60^\circ$ and $\Omega = 0.015$. The corresponding mean-field dynamics are shown by the gray curves. All quantities are dimensionless.

of the transverse momentum and angular momentum, we consider three representative cases: (i) $S = 0$, $\Omega = 0.15$, (ii) $S = 4$, $\Omega = 0.01$, and (iii) $S = 4$, $\Omega = 0.015$, $\theta = 60^\circ$. For each case, we also present the corresponding mean-field dynamics to highlight the deviation between mean-field

and many-body results. The results are shown in Fig. S5. Figures S5(a) and S5(b) depict the time evolution of the transverse momentum per particle, $\langle P_y \rangle$ and the angular momentum per particle $\langle L_z \rangle$ for a centered double well with $S = 0$, $\Omega = 0.15$. The gray curves represent the corresponding mean-field dynamics. While the mean-field results exhibit oscillations with constant amplitude, the many-body dynamics in both cases show a clear damping of the oscillations. Figures S5(c) and S5(d) present the corresponding dynamics of these two quantities for an off-centered double well. For demonstration, we choose the parameters $S = 0$, $\Omega = 0.01$. Figures S5(e) and S5(f) show the corresponding dynamics of the same two quantities for an off-centered and oriented double-well potential. For illustration, we choose the parameters $S = 4$, $\Omega = 0.015$, and $\theta = 60°$. All the observations exhibit that the many-body dynamics show damped oscillations in both $\langle P_y \rangle$ and $\langle L_z \rangle$, whereas the mean-field results display undamped, persistent oscillations. This damping in the many-body case arises because the depletion grows over time. The system starts from a highly condensed state, so during the short-time evolution the mean-field and many-body results almost coincide. The differences become significant at longer times, when fragmentation becomes substantial.

[1] O. E. Alon, A. I. Streltsov, and L. S. Cederbaum, *Multiconfigurational time-dependent Hartree method for bosons: Many-body dynamics of bosonic systems*, Phys. Rev. A **77**, 033613 (2008).

[2] R. Roy, S. Dutta, and O. E. Alon, *Rotation quenches in trapped bosonic systems*, Sci. Rep. **15**, 27193 (2025).

[3] A. U. J. Lode, C. Lévêque, L. B. Madsen, A. I. Streltsov, and O. E. Alon, *Colloquium: Multiconfigurational time-dependent Hartree approaches for indistinguishable particles*, Rev. Mod. Phys. **92**, 011001 (2020).

[4] R. Roy and O. E. Alon, *Assessing small accelerations using a bosonic Josephson junction*, Phys. Rev. A **111**, 043307 (2025).

[5] S. Klaiman and O. E. Alon, *Variance as a sensitive probe of correlations*, Phys. Rev. A **91**, 063613 (2015).

[6] O. E. Alon, *Analysis of a trapped Bose–Einstein condensate in terms of position, momentum, and angular-momentum variance*, Symmetry **11**, 1344 (2019).
